# Supplementary material for: Conductance Quantization at zero magnetic field in InSb nanowires
Source: arXiv:1603.03751 ancillary file (2016-03-11)
Supplement: Supplementary file 1 [file Supplementary-Materials-arxiv.pdf]

# Supporting information for: Conductance Quantization at zero magnetic field in InSb nanowires

Jakob Kammhuber,[†] Maja C. Cassidy,[†] Hao Zhang,[†] Önder Gül,[†] Fei Pei,[†] Michiel W. A. de Moor,[†] Bas Nijholt,[†] Kenji Watanabe,[‡] Takashi Taniguchi,[‡] Diana Car,[¶] Sébastien R. Plissard,[†,¶,§] Erik P. A. M. Bakkers,[†,¶] and Leo P. Kouwenhoven[*,†]

*QuTech and Kavli Institute of Nanoscience, Delft University of Technology, 2628 CJ Delft, The Netherlands, Advanced Materials Laboratory, National Institute for Materials Science, 1-1 Namiki, Tsukuba, 305-0044, Japan, Department of Applied Physics, Eindhoven University of Technology, 5600 MB Eindhoven, The Netherlands, and CNRS-Laboratoire d'Analyse et d'Architecture des Systemes (LAAS), Université de Toulouse, 7 avenue du Colonel Roche, F-31400 Toulouse, France*

E-mail: l.p.kouwenhoven@tudelft.nl

[*]To whom correspondence should be addressed

[†]QuTech and Kavli Institute of Nanoscience, Delft University of Technology, 2628 CJ Delft, The Netherlands

[‡]Advanced Materials Laboratory, National Institute for Materials Science, 1-1 Namiki, Tsukuba, 305-0044, Japan

[¶]Department of Applied Physics, Eindhoven University of Technology, 5600 MB Eindhoven, The Netherlands

[§]Current address: CNRS-Laboratoire d'Analyse et d'Architecture des Systemes (LAAS), Université de Toulouse, 7 avenue du Colonel Roche, F-31400 Toulouse, France

## Fabrication Recipe

**Substrate preparation** : Intrinsic Si with 285 nm thermal $SiO_2$ and alignment markers made of 10 nm Ti + 80 nm Au was used as substrate.

**Fine gate deposition** :

- Resist spinning: PMMA 950 K A2 at 5000 rpm; bake for 60 min at 175 °C
- Writing of gate patterns using ebeam lithography.
- Developing: 60 s MIBK:IPA (1:3); 60 s IPA.
- Deposition: Evaporation of 5 nm Ti and 10 nm Au.
- Lift-off in hot (50 °C) Acetone for 2 hours.

**Dielectric deposition** : Hexagonal boron nitride (hBN) was transferred on top of the fine gates in a setup similar to Ref S1 which also contains a more detailed description of the process.

- Exfoliated hBN flakes are transferred on a glass substrates covered with a PDMS film.
- Identification of fitting hBN flakes (20 - 25 nm typical thickness), alignment to the fine gates and transfer onto the chip are all done with an optical microscope.
- Cleaning of PDMS residues with oxygen plasma (60 s, 1 mBar, 600 W).

**Wire deposition** : InSb nanowires are transferred onto the chip with fine gates covered by hBN under an optical microscope equipped with a fine needle (250 nm diameter) attached to a micro-manipulator similar to the setup described in Ref S2.

**Contact deposition** :

- SEM imaging of nanowires for contact design.
- Resist spinning: PMMA 950 K A4 at 4000 rpm; bake for 15 min at 175 °C.

- Writing of contact patterns using ebeam lithography.
- Developing: 60 s MIBK:IPA (1:3); 60 s IPA.
- Sulfur passivation as described in ref. S3: Diluted ammonium polysulfide $(NH_4)_2S_x$ solution (3.5 ml $(NH_4)_2S$ mixed with 290 mg sulfur then diluted with DI-water at a ration of 1 : 200) for 30 min at 60 °C. Rinse in DI water and transfer chip to the evaporator in a non-transparent beaker filled with IPA.
- 30 s He-etch with a Kauffman ion source.
- Deposition: Evaporation of 10 nm Cr and 90 nm Au.
- Lift-off in hot (50 °C) Acetone for 2 h.

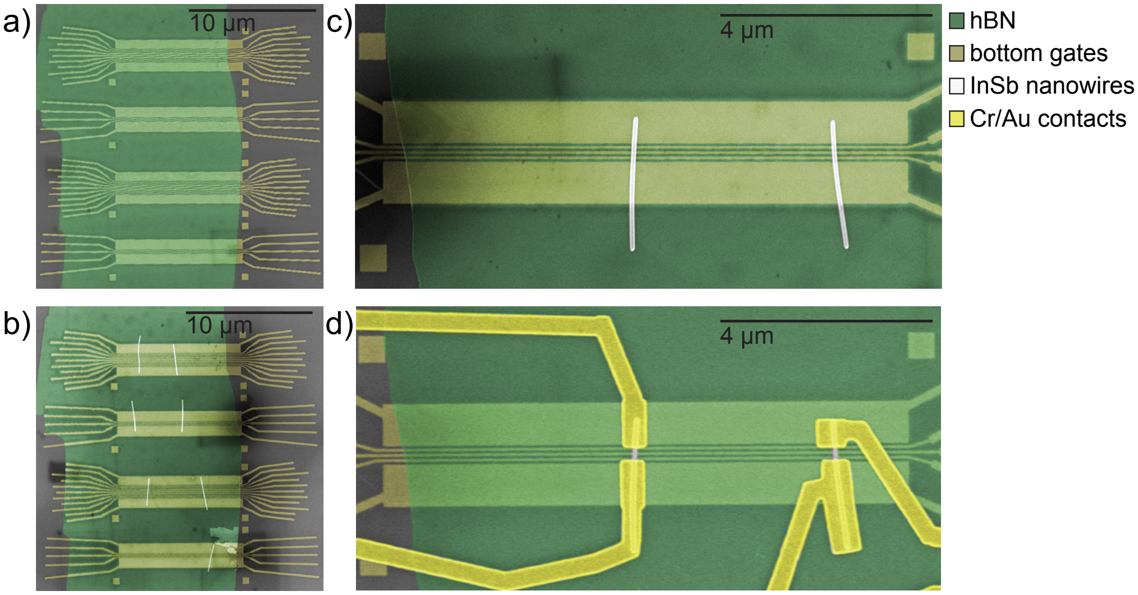


Figure S1: False color SEM images illustrating the fabrication process. (a) Ti/Au bottom gates (dark yellow) with a hBN flake (green) on top. (b),(c) InSb nanowires (white) deposited on hBN and aligned perpendicular to the fine gates. (d) Two finished devices after evaporation of Cr/Au contacts (light yellow).

## Contact Resistance

After subtracting a series resistance of 5.6 kΩ for filters and 3 kΩ for the measurement setup all data was corrected for an additional device dependent contact resistance $R_{device}$. This accounts for the resistance of the metallic contacts as well as the resistance of the metal-nanowire interface. $R_{device}$ was chosen to fit the height of the 1 $G_0$-plateau to $2e^2/h$ at high magnetic fields B = 5 T and then used for all other scans of the same device. Typical values of $R_{device}$ are 3 - 6 kΩ and for the main device presented in Fig. $2-5$ of the main text we subtracted $R_{device} = 6.5\,k\Omega$.

## Numerical Simulations

Numerical Simulations of the sub-band dispersion have been performed using the Kwant code[S4] with the model described in ref S5. The model consisted of a hexagonal nanowire with radius r = 35 nm and g-factor g = 40 and includes spin orbit interaction as well as orbital effects. The source code can be found in the supplementary materials of ref S5.

## Additional data of main device and lever arm extraction

In addition to the data shown in the main text we also took measurements at intermediate values of magnetic field. Conductance, transconductance and gate traces as function of bias voltage and gate voltage are shown in Figures S3 and S4. From this we extracted the gate lever arm $\eta$ via $V_{gate}\eta = \Delta E_{subband}$ and find $\eta = 40 \pm 3\,meV/V$. The data also shows that higher conductance plateaus are not always clearly resolved in the low bias lock-in measurements. We also observe this in other devices and it is probably due to remaining imperfections in the device which show up stronger in the less-averaging low bias measurements.

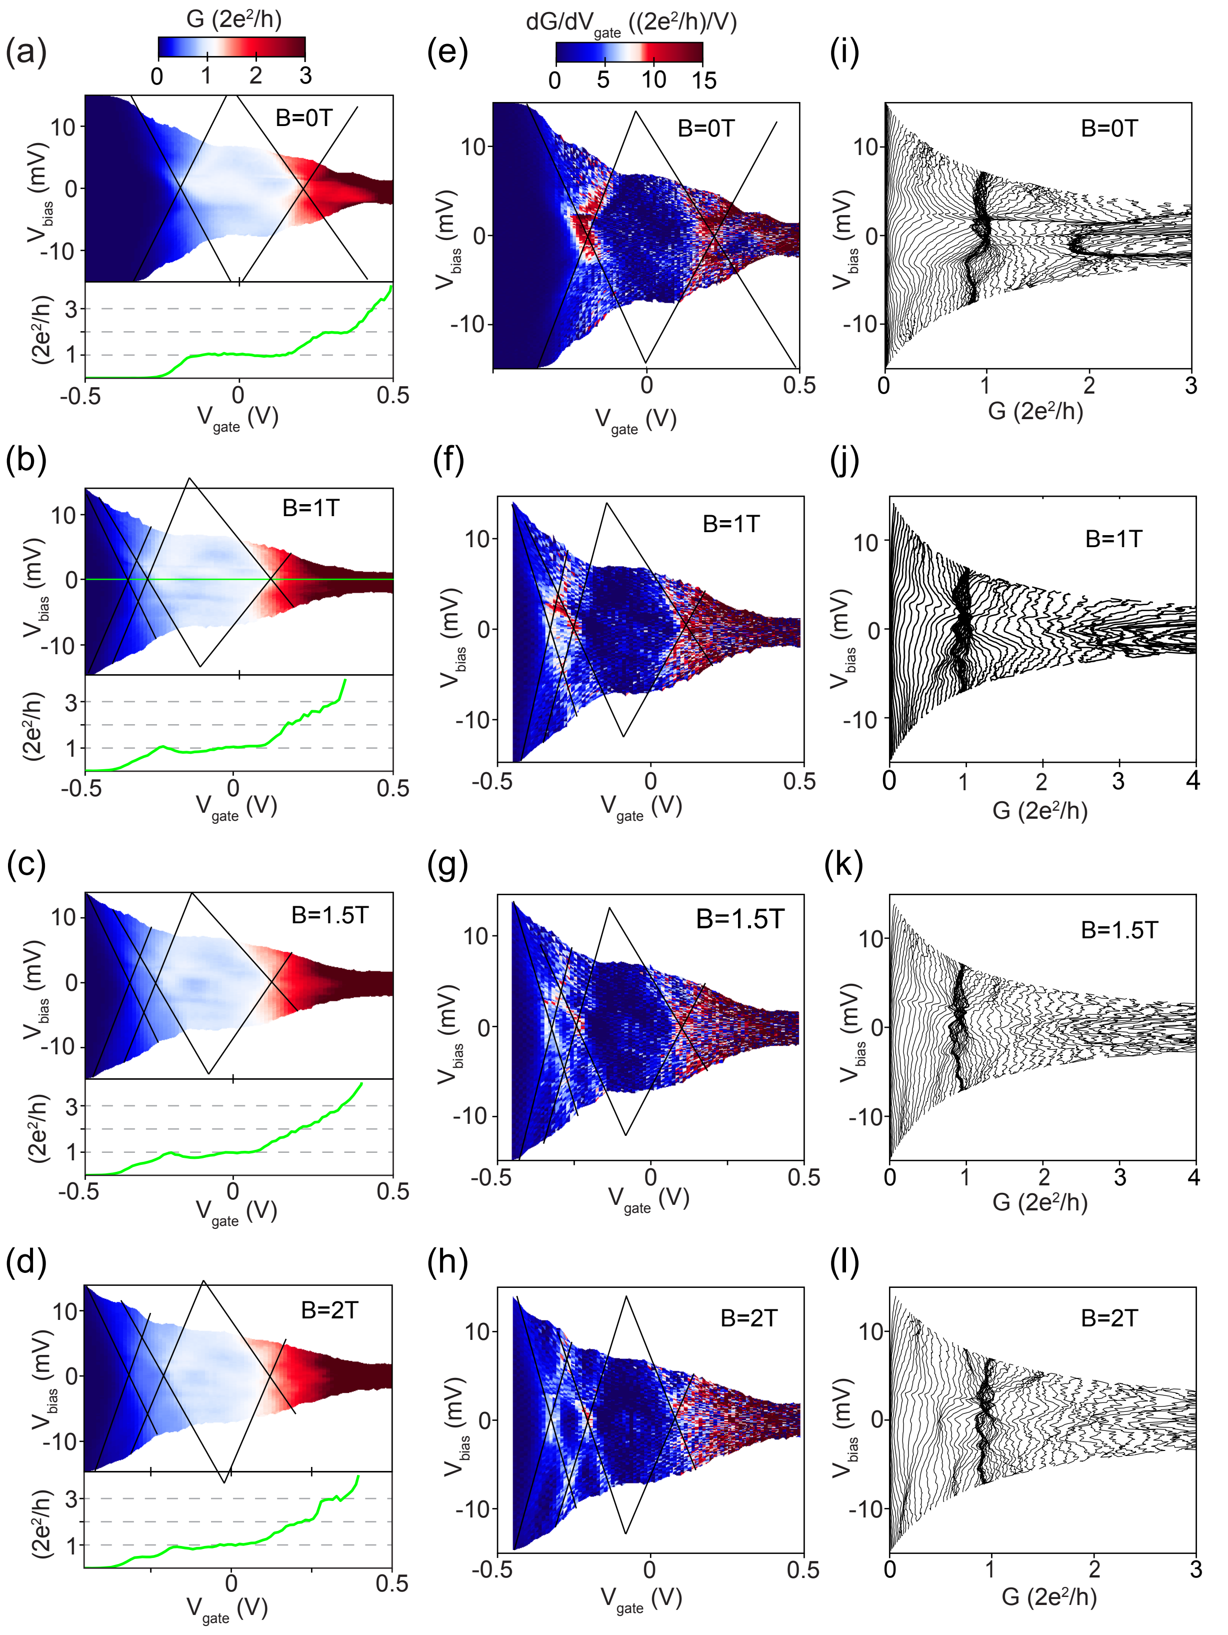


Figure S2: (a)-(d) Differential conductance G as function of $V_{bias}$ and $V_{gate}$ at increasing magnetic fields. (e)-(h) transconductance $dG/dV_{gate}$ at increasing magnetic fields. (i)-(l) Line cuts from a)-d) at fixed $V_{gate}$ drawn without offset between individual traces.

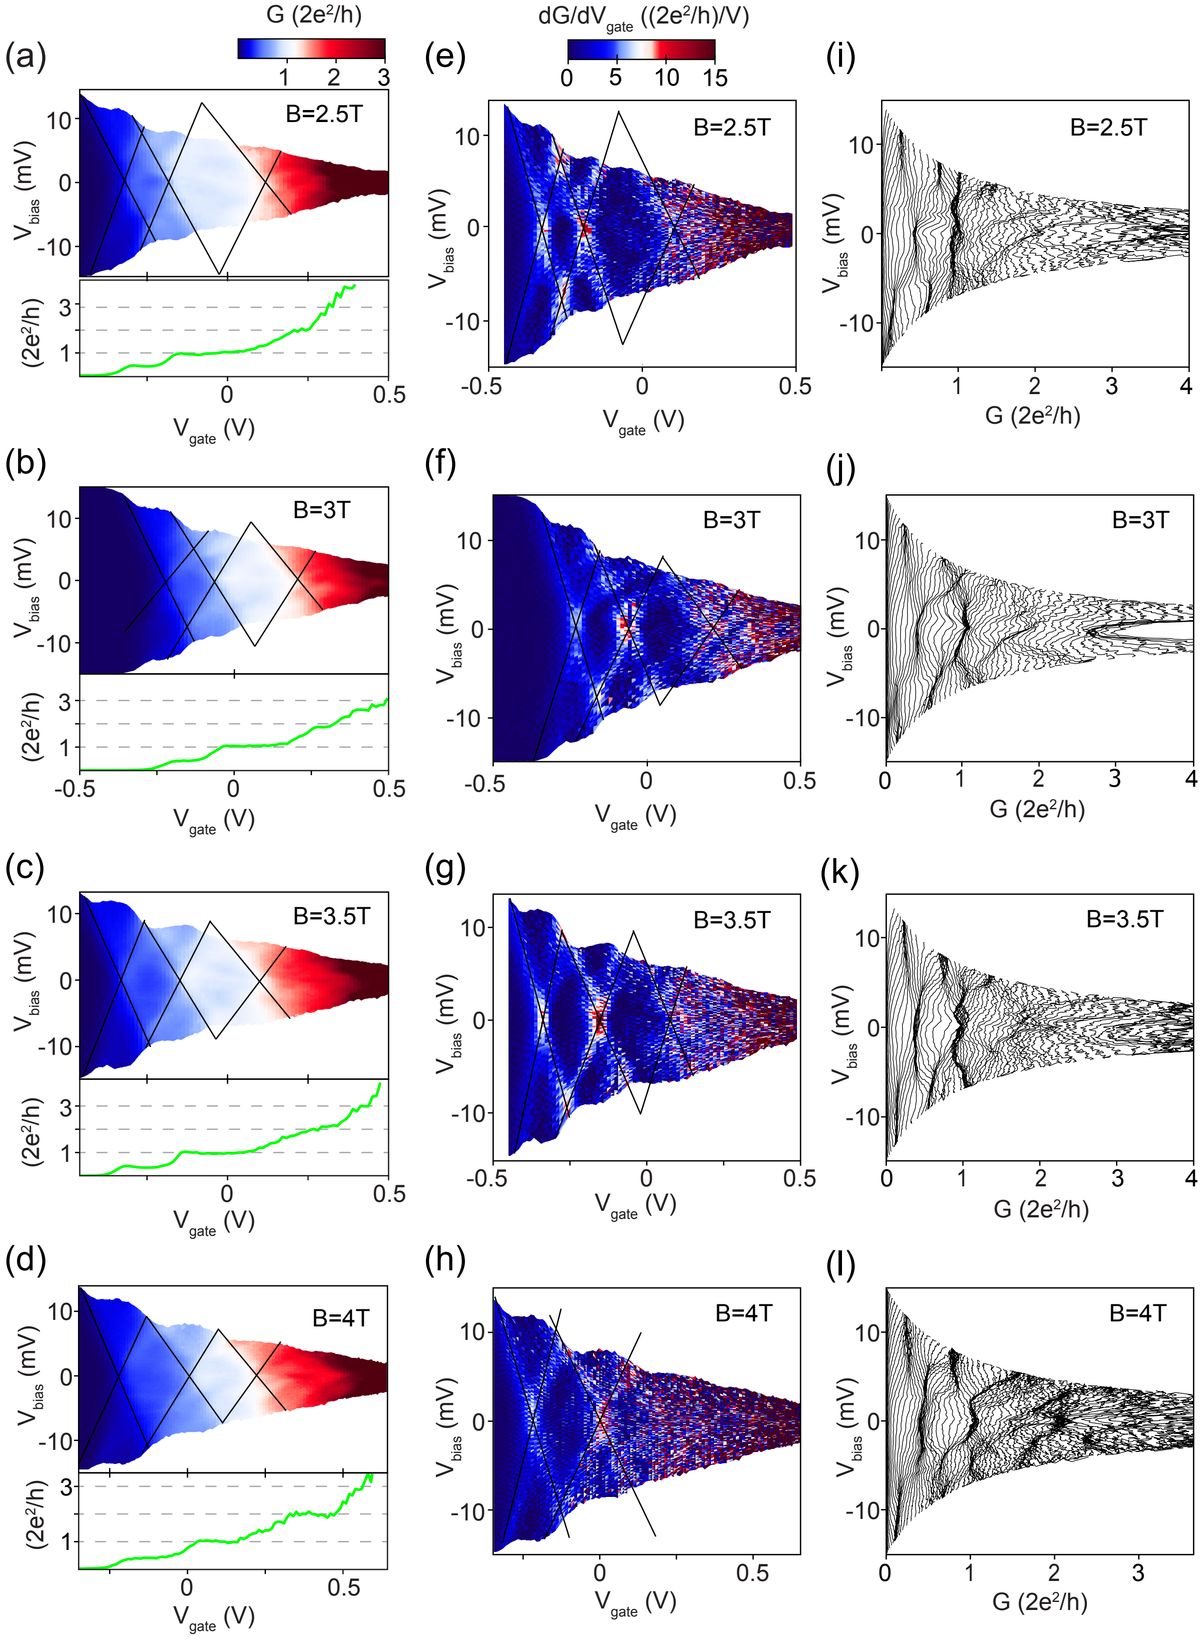

Figure S3: (a)-(d) Differential conductance G as function of $V_{bias}$ and $V_{gate}$ at increasing magnetic fields. (e)-(h) transconductance $dG/dV_{gate}$ at increasing magnetic fields. (i)-(l) Line cuts from a)-d) at fixed $V_{gate}$ drawn without offset between individual traces.

# Data of additional devices

All together we fabricated eight working devices on the same chip and data for four of those is shown in Fig 1 of the main text. For completeness the I-V traces of all eight devices is shown in Fig S4. As mentioned in the main text devices with both fine and wide bottom gates were fabricated. Fine gates had a width of 50 nm and pitch of 100 nm, wide gates had a width of 800 nm effectively extending through the full QPC channel and under the metallic contacts. Fine gates allow more flexibility in gating, but the gate potential will be less homogeneous (when using multiple fine gates) with a sharper onset. This can increase the chance of back reflection and give more pronounced Fabry Perot oscillations. Wide bottom gates on the other hand have a smoother onset of the potential profile which increases the QPC transmission and visibility. Data of an additional device with fine gates is shown in Fig S5.

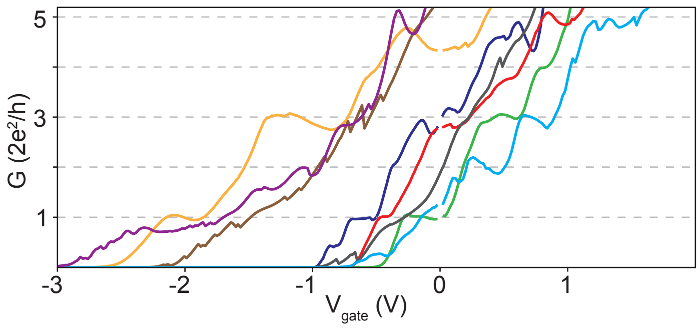


Figure S4: I-V traces of all eight fabricated devices with hBN dielectric.

# Devices fabricated on $SiO_2$ dielectric

To compare the influence of the gate dielectric we also fabricated identical devices with of nanowires deposited on highly doped Si++ with 285 nm $SiO_2$ as dielectric. These devices also showed clear signs of conductance quantization as demonstrated in Fig S6. Data of quantum point contacts with identical contact spacing but different dielectric is shown in Fig S7 which verifies the improvements due to the hBN dielectric.

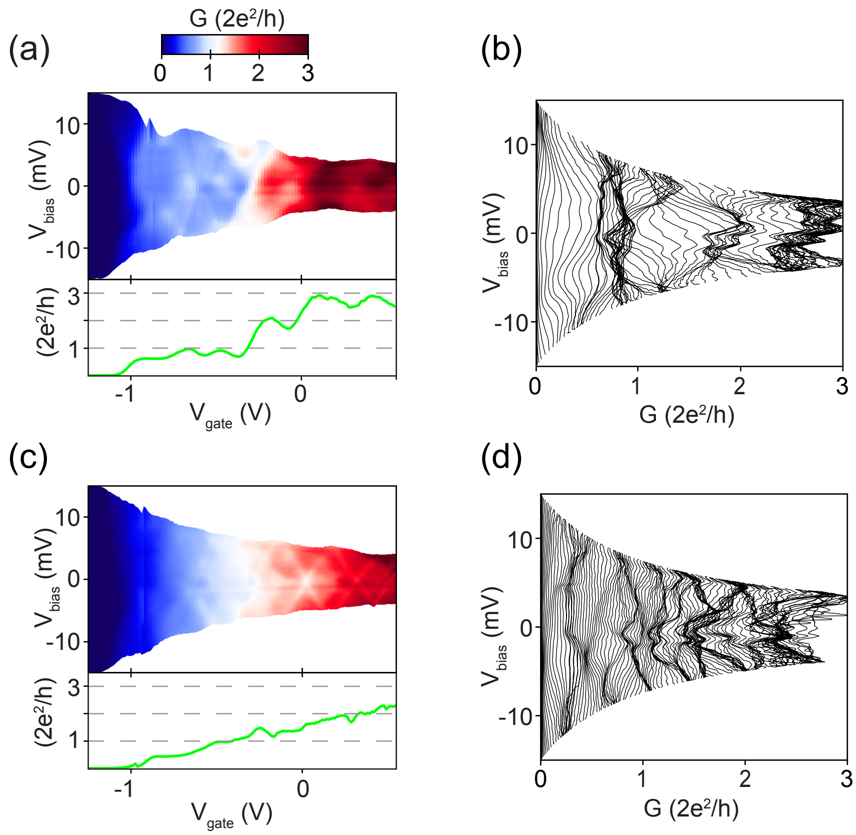


Figure S5: a,b) Differential conductance G of a second device on hBN and with fine gates at B $= 0T$ (a) and B $= 4T$ (b) c,d) Line-cuts from a,b) at fixed $V_{gate}$ drawn without offset.

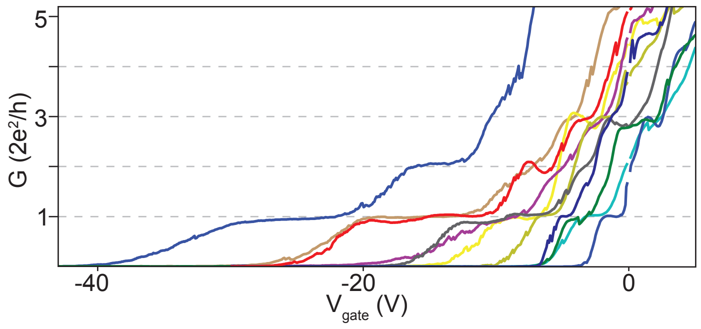


Figure S6: I-V traces of 11 different devices with wires on a $SiO_2$ dielectric taken at $V_{bias} =$ 10 mV

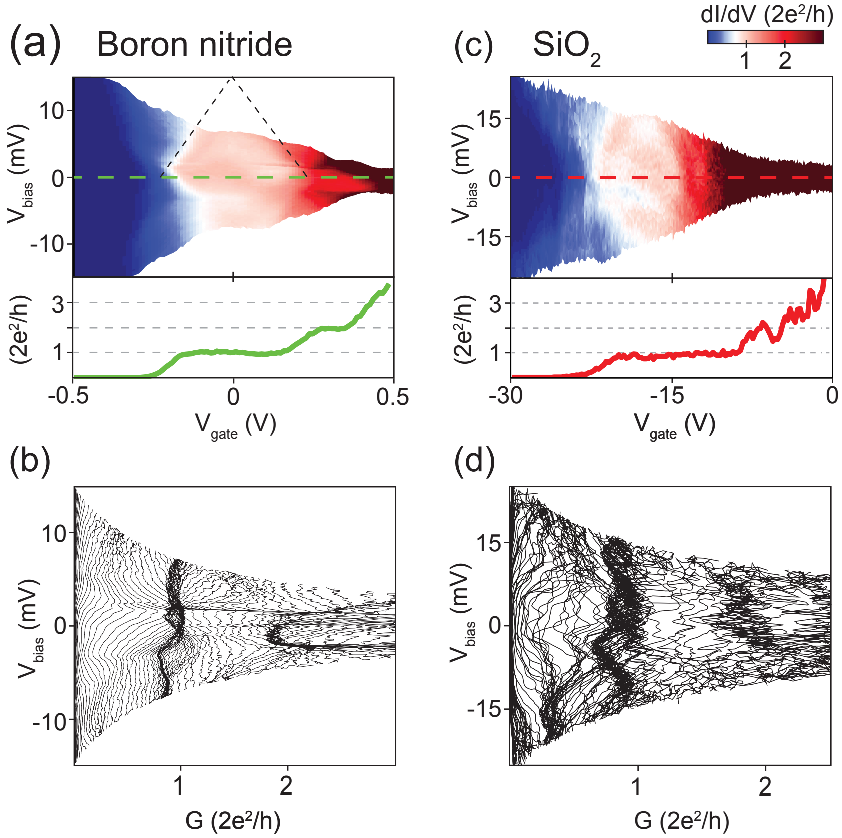


Figure S7: (a)Color plot of the differential conductance G as function of $V_{bias}$ and $V_{gate}$ for a device with hBN dielectric at B = 0 T. A line cut along $V_{bias}$ = 0 mV is shown in the bottom panel. (b) Line traces from a) at fixed $V_{gate}$ drawn without offset between individual traces. (c) Color plot of the differential conductance G as function of $V_{bias}$ and $V_{gate}$ of a device with a $SiO_2$ dielectric. (d) Line traces of c) at fixed $V_{gate}$.

## References


(S1) Castellanos-Gomez, A.; Buscema, M.; Molenaar, R.; Singh, V.; Janssen, L.; van der Zant, H. S. J.; Steele, G. A. *2D Mater.* **2014**, *1*, 011002.

(S2) Flöhr, K.; Liebmann, M.; Sladek, K.; Günel, H. Y.; Frielinghaus, R.; Haas, F.; Meyer, C.; Hardtdegen, H.; Schäpers, T.; Grützmacher, D.; Morgenstern, M. *Rev. Sci. Instrum.* **2011**, *82*, 113705.

(S3) Suyatin, D. B.; Thelander, C.; Björk, M. T.; Maximov, I.; Samuelson, L. *Nanotechnology* **2007**, *18*, 105307.

(S4) Groth, C. W.; Wimmer, M.; Akhmerov, A. R.; Waintal, X. *New J. Phys.* **2014**, *16*, 063065.

(S5) Nijholt, B.; Akhmerov, A. R. *arXiv:1509.02675* **2015**,
